# Supplementary material for: Exploring the Landscape of Machine Unlearning: A Comprehensive Survey and Taxonomy
Source: arXiv:2305.06360 source file (2024-02-01)
Supplement: Supplementary file 1 [file Supplementary_Material.pdf]

# Exploring the Landscape of Machine Unlearning: A Comprehensive Survey and Taxonomy (Supplementary Material)

Thanveer Shaik, Xiaohui Tao, Haoran Xie, Lin Li, Xiaofeng Zhu, and Qing Li

## SUPPLEMENTARY MATERIAL

In this section, we present supplementary details for Table IV “Public Datasets for Machine Unlearning” in the survey, which includes an approximation of their popularity based on the frequency of their references. The popularity of datasets is classified into three categories, namely, “High”, “Moderate”, or “Low”, depending on the frequency they were referenced. Specifically, a dataset is considered highly popular if it was referred to in seven or more sources, moderately popular if it

appeared in four to six sources, and poorly popular if it was mentioned in three or fewer sources.

TABLE I  
PUBLIC DATASETS FOR MACHINE UNLEARNING WITH SUPPLEMENTARY INFORMATION FOR POPULARITY

| Modality        | Dataset                          | No. of Instances | No. of Attributes | Task                    | Popularity | References       | References Count |
|-----------------|----------------------------------|------------------|-------------------|-------------------------|------------|------------------|------------------|
| Image           | SVHN [1]                         | 600,000          | 3072              | Object recognition      | High       | [2]–[10]         | 9                |
|                 | CIFAR-100 [11]                   | 60,000           | 3072              | Object recognition      | High       | [12]–[18]        | 7                |
|                 | Imagenet [19]                    | 1.2 million      | 1,000             | Object recognition      | Medium     | [20]–[23]        | 4                |
|                 | Mini-Imagenet [24]               | 100,000          | 784               | Object recognition      | Low        | [25]             | 1                |
|                 | LSUN [26]                        | 1.2 million      | varies            | Scene recognition       | Low        | [27], [28]       | 2                |
|                 | MNIST [29]                       | 70,000           | 784               | Object recognition      | High       | [20], [30]–[48]  | 20               |
| Text            | IMDB [49]                        | 50,000           | varies            | Sentiment analysis      | Medium     | [50]–[54]        | 5                |
|                 | Newsgroup [55]                   | 19,188           | varies            | Text classification     | Low        | [56]             | 1                |
|                 | Reuters [57]                     | 10,788           | varies            | Text classification     | Low        | [58], [59]       | 2                |
|                 | SQuAD [60]                       | 100,000          | Varies            | Question answering      | Low        | [61]–[63]        | 3                |
| Tabular         | Adult [64]                       | 48,842           | 14                | Income prediction       | Low        | [65]–[67]        | 3                |
|                 | Breast Cancer [68]               | 286              | 9                 | Cancer diagnosis        | Low        | [69], [70]       | 2                |
|                 | Diabetes [71]                    | 768              | 8                 | Diabetes diagnosis      | Low        | [72], [73]       | 2                |
| Time series     | Epileptic Seizure [74]           | 11,500           | 178               | Seizure prediction      | Low        | [32], [75]       | 2                |
|                 | Activity Recognition [76]        | 10,299           | 561               | Activity Classification | Low        | [75], [77], [78] | 3                |
| Graph           | OGB [79]                         | 1.2 million      | varies            | Graph classification    | Low        | [80]             | 1                |
|                 | Cora [81]                        | 2,708            | 1,433             | Graph classification    | Low        | [82], [83]       | 2                |
|                 | Yelp Dataset [84]                | 8,282,442        | Varies            | Recommendation          | Low        | [85], [86]       | 2                |
| Computer Vision | Fashion-MNIST [87]               | 70,000           | 784               | Image classification    | Medium     | [88]–[91]        | 4                |
|                 | Caltech-101 [92]                 | 9,146            | Varies            | Object recognition      | Low        | [93]–[95]        | 3                |
|                 | COCO [96]                        | 330,000          | Varies            | Object detection        | Medium     | [97]–[101]       | 5                |
|                 | YouTube Faces [102]              | 3,425            | 2,622             | Face recognition        | Medium     | [103]–[107]      | 5                |
|                 | EuroSAT [108]                    | 27,000           | 13                | Land use classification | Low        | [10], [109]      | 2                |
| Transaction     | Purchase [110]                   | 39,624           | 8                 | Purchase prediction     | Medium     | [111]–[115]      | 5                |
| Sequence        | Human Activity Recognition [116] | 10,299           | 561               | Activity recognition    | Low        | [117]            | 1                |
| Recommendation  | MovieLens [118]                  | 100,000          | varies            | Movie recommendation    | High       | [119]–[125]      | 7                |

## REFERENCES

- [1] Y. Netzer, T. Wang, A. Coates, A. Bissacco, B. Wu, and A. Y. Ng, "Reading digits in natural images with unsupervised feature learning," in *NIPS Workshop on Deep Learning and Unsupervised Feature Learning*, 2011.
- [2] Z. Zhang, Y. Zhou, X. Zhao, T. Che, and L. Lyu, "Prompt certified machine unlearning with randomized gradient smoothing and quantization," in *Advances in Neural Information Processing Systems* (S. Koyejo, S. Mohamed, A. Agarwal, D. Belgrave, K. Cho, and A. Oh, eds.), vol. 35, pp. 13433–13455, Curran Associates, Inc., 2022.
- [3] J. Jia, J. Liu, P. Ram, Y. Yao, G. Liu, Y. Liu, P. Sharma, and S. Liu, "Model sparsification can simplify machine unlearning," *arXiv preprint arXiv:2304.04934*, 2023.
- [4] B. Casella, A. B. Chisari, S. Battiato, and M. V. Giuffrida, "Transfer learning via test-time neural networks aggregation," *arXiv preprint arXiv:2206.13399*, 2022.
- [5] A. Setlur, B. Eysenbach, V. Smith, and S. Levine, "Adversarial unlearning: Reducing confidence along adversarial directions," *arXiv preprint arXiv:2206.01367*, 2022.
- [6] Y. Li, Y. Jiang, Z. Li, and S.-T. Xia, "Backdoor learning: A survey," *IEEE Transactions on Neural Networks and Learning Systems*, 2022.
- [7] L. Feng, Z. Qian, S. Li, and X. Zhang, "Trojaning semi-supervised learning model via poisoning wild images on the web," *arXiv preprint arXiv:2301.00435*, 2023.
- [8] A. S. Rakin, Z. He, and D. Fan, "Tbt: Targeted neural network attack with bit trojan," in *Proceedings of the IEEE/CVF Conference on Computer Vision and Pattern Recognition*, pp. 13198–13207, 2020.
- [9] P. Pathak, J. Zhang, and D. Samaras, "Local learning on transformers via feature reconstruction," *arXiv preprint arXiv:2212.14215*, 2022.
- [10] J. Loedeman, M. C. Stol, T. Han, and Y. M. Asano, "Prompt generation networks for efficient adaptation of frozen vision transformers," *arXiv preprint arXiv:2210.06466*, 2022.
- [11] A. Krizhevsky, G. Hinton, et al., "Learning multiple layers of features from tiny images," 2009.
- [12] Y. Dukler, B. Bowman, A. Achille, A. Golatkar, A. Swaminathan, and S. Soatto, "Safe: Machine unlearning with shard graphs," *arXiv preprint arXiv:2304.13169*, 2023.
- [13] A. Thudi, G. Deza, V. Chandrasekaran, and N. Papernot, "Unrolling sgd: Understanding factors influencing machine unlearning," in *2022 IEEE 7th European Symposium on Security and Privacy (EuroS&P)*, pp. 303–319, IEEE, 2022.
- [14] A. Mahadevan and M. Mathioudakis, "Certifiable unlearning pipelines for logistic regression: An experimental study," *Machine Learning and Knowledge Extraction*, vol. 4, no. 3, pp. 591–620, 2022.
- [15] Y. Jiang, S. Liu, T. Zhao, W. Li, and X. Gao, "Machine unlearning survey," in *Fifth Int'l conf. on Mechatronics and Computer Technology Engineering (MCTE 2022)*, vol. 12500, pp. 1596–1603, SPIE, 2022.
- [16] M. Chen, W. Gao, G. Liu, K. Peng, and C. Wang, "Boundary unlearning," *arXiv preprint arXiv:2303.11570*, 2023.
- [17] X. Gao, X. Ma, J. Wang, Y. Sun, B. Li, S. Ji, P. Cheng, and J. Chen, "Verifi: Towards verifiable federated unlearning," *arXiv preprint arXiv:2205.12709*, 2022.
- [18] N. Carlini, F. Tramèr, E. Wallace, M. Jagielski, A. Herbert-Voss, K. Lee, A. Roberts, T. B. Brown, D. Song, U. Erlingsson, et al., "Extracting training data from large language models," in *USENIX Security Symposium*, vol. 6, 2021.
- [19] J. Deng, W. Dong, R. Socher, L.-J. Li, K. Li, and L. Fei-Fei, "Imagenet: A large-scale hierarchical image database," in *2009 IEEE conference on computer vision and pattern recognition*, pp. 248–255, Ieee, 2009.
- [20] S. Poppi, S. Sarto, M. Cornia, L. Baraldi, and R. Cucchiara, "Multi-class explainable unlearning for image classification via weight filtering," *arXiv preprint arXiv:2304.02049*, 2023.
- [21] S. Cha, S. Cho, D. Hwang, H. Lee, T. Moon, and M. Lee, "Learning to unlearn: Instance-wise unlearning for pre-trained classifiers," *arXiv preprint arXiv:2301.11578*, 2023.
- [22] W. Chen, B. Wu, and H. Wang, "Effective backdoor defense by exploiting sensitivity of poisoned samples," *Advances in Neural Information Processing Systems*, vol. 35, pp. 9727–9737, 2022.
- [23] S. Shan, W. Ding, E. Wenger, H. Zheng, and B. Y. Zhao, "Post-breach recovery: Protection against white-box adversarial examples for leaked dnn models," in *Proceedings of the 2022 ACM SIGSAC Conference on Computer and Communications Security*, pp. 2611–2625, 2022.
- [24] O. Vinyals, C. Blundell, T. Lillicrap, D. Wierstra, et al., "Matching networks for one shot learning," *Advances in neural information processing systems*, vol. 29, 2016.
- [25] M. Riemer, I. Cases, R. Ajemian, M. Liu, I. Rish, Y. Tu, and G. Tesauero, "Learning to learn without forgetting by maximizing transfer and minimizing interference," *arXiv preprint arXiv:1810.11910*, 2018.
- [26] F. Yu, Y. Zhang, S. Song, A. Seff, and J. Xiao, "Lsun: Construction of a large-scale image dataset using deep learning with humans in the loop," *arXiv preprint arXiv:1506.03365*, 2015.
- [27] Z. Li, A. Hoogs, and C. Xu, "Discover and mitigate unknown biases with debiasing alternate networks," in *Computer Vision—ECCV 2022: 17th European Conference, Tel Aviv, Israel, October 23–27, 2022, Proceedings, Part XIII*, pp. 270–288, Springer, 2022.
- [28] Y. Zhou and I. Nwogu, "Learning to generate high resolution images with bilateral adversarial networks," in *Proceedings of the Int'l conf. on Advances in Image Processing*, pp. 113–117, 2017.
- [29] Y. LeCun, L. Bottou, Y. Bengio, and P. Haffner, "Gradient-based learning applied to document recognition," *Proceedings of the IEEE*, vol. 86, no. 11, pp. 2278–2324, 1998.
- [30] L. Bourtole, V. Chandrasekaran, C. A. Choquette-Choo, H. Jia, A. Travers, B. Zhang, D. Lie, and N. Papernot, "Machine unlearning," in *2021 IEEE Symposium on Security and Privacy (SP)*, May 2021.
- [31] V. Gupta, C. Jung, S. Neel, A. Roth, S. Sharifi-Malvajerdi, and C. Waites, "Adaptive machine unlearning," *Advances in Neural Information Processing Systems*, vol. 34, pp. 16319–16330, 2021.
- [32] T. T. Nguyen, T. T. Huynh, P. L. Nguyen, A. W.-C. Liew, H. Yin, and Q. V. H. Nguyen, "A survey of machine unlearning," *arXiv preprint arXiv:2209.02299*, 2022.
- [33] D. M. Sommer, L. Song, S. Wagh, and P. Mittal, "Towards probabilistic verification of machine unlearning," *arXiv preprint arXiv:2003.04247*, 2020.
- [34] V. S. Chundawat, A. K. Tarun, M. Mandal, and M. Kankanhalli, "Zero-shot machine unlearning," *arXiv preprint arXiv:2201.05629*, 2022.
- [35] T. Baumhauer, P. Schöttle, and M. Zeppelzauer, "Machine unlearning: Linear filtration for logit-based classifiers," *Machine Learning*, vol. 111, no. 9, pp. 3203–3226, 2022.
- [36] N. G. Marchant, B. I. Rubinstein, and S. Alfeld, "Hard to forget: Poisoning attacks on certified machine unlearning," in *Proc. of the AAAI Conf. on Artificial Intelligence*, vol. 36, pp. 7691–7700, 2022.
- [37] Z. Lu, H. Liang, M. Zhao, Q. Lv, T. Liang, and Y. Wang, "Label-only membership inference attacks on machine unlearning without dependence of posteriors," *Int'l Journal of Intelligent Systems*, vol. 37, no. 11, pp. 9424–9441, 2022.
- [38] P.-F. Zhang, G. Bai, Z. Huang, and X.-S. Xu, "Machine unlearning for image retrieval: A generative scrubbing approach," in *Proceedings of the 30th ACM Int'l conf. on Multimedia*, pp. 237–245, 2022.
- [39] A. Becker and T. Liebig, "Evaluating machine unlearning via epistemic uncertainty," *arXiv preprint arXiv:2208.10836*, 2022.
- [40] Z. Zhou, X. Liu, J. Li, J. Ruan, and M. Fan, "Dynamically selected mixup machine unlearning," in *2022 IEEE Int'l conf. on Trust, Security and Privacy in Computing and Communications (TrustCom)*, pp. 514–524, IEEE, 2022.
- [41] K. Chen, Y. Wang, and Y. Huang, "Lightweight machine unlearning in neural network," *arXiv preprint arXiv:2111.05528*, 2021.
- [42] Y. Yoon, J. Nam, H. Yun, D. Kim, and J. Ok, "Few-shot unlearning by model inversion," *arXiv preprint arXiv:2205.15567*, 2022.
- [43] A. Halimi, S. Kadhe, A. Rawat, and N. Baracaldo, "Federated unlearning: How to efficiently erase a client in fl?," *arXiv preprint arXiv:2207.05521*, 2022.
- [44] C. Wu, S. Zhu, and P. Mitra, "Federated unlearning with knowledge distillation," *arXiv preprint arXiv:2201.09441*, 2022.
- [45] Y. Fraboni, R. Vidal, L. Kameni, and M. Lorenzi, "Sequential informed federated unlearning: Efficient and provable client unlearning in federated optimization," *arXiv preprint arXiv:2211.11656*, 2022.
- [46] Z. Lu, Y. Wang, Q. Lv, M. Zhao, and T. Liang, "Fp 2-mia: A membership inference attack free of posterior probability in machine unlearning," in *Provable and Practical Security: 16th Int'l conf., ProvSec 2022, Nanjing, China, November 11–12, 2022, Proceedings*, pp. 167–175, Springer, 2022.
- [47] J. Gao, S. Garg, M. Mahmood, and P. N. Vasudevan, "Deletion inference, reconstruction, and compliance in machine (un) learning," *arXiv preprint arXiv:2202.03460*, 2022.
- [48] J. Stock, J. Wettlaufer, D. Demmler, and H. Federrath, "Property unlearning: A defense strategy against property inference attacks," *arXiv preprint arXiv:2205.08821*, 2022.
- [49] A. L. Maas, R. E. Daly, P. T. Pham, D. Huang, A. Y. Ng, and C. Potts, "Learning word vectors for sentiment analysis," in *Proceedings of the 49th Annual Meeting of the Association for Computational Linguistics*:

- Human Language Technologies*, (Portland, Oregon, USA), pp. 142–150, Association for Computational Linguistics, June 2011.
- [50] E. Chien, C. Pan, and O. Milenkovic, “Certified graph unlearning,” *arXiv preprint arXiv:2206.09140*, 2022.
  - [51] R. Zhu, D. Tang, S. Tang, X. Wang, and H. Tang, “Selective amnesia: On efficient, high-fidelity and blind suppression of backdoor effects in trojaned machine learning models,” *arXiv preprint arXiv:2212.04687*, 2022.
  - [52] M. Abolfazli, A. Host-Madsen, and J. Zhang, “Differential description length for hyperparameter selection in machine learning,” *arXiv preprint arXiv:1902.04699*, 2019.
  - [53] A. R. Nelakurthi, R. Maciejewski, and J. He, “Source free domain adaptation using an off-the-shelf classifier,” in *2018 IEEE Int’l conf. on big data (Big Data)*, pp. 140–145, IEEE, 2018.
  - [54] D. Friedman, A. Wettig, and D. Chen, “Finding dataset shortcuts with grammar induction,” *arXiv preprint arXiv:2210.11560*, 2022.
  - [55] T. Joachims, “A probabilistic analysis of the rocchio algorithm with tfidf for text categorization,” tech. rep., Carnegie-mellon univ pittsburgh pa dept of computer science, 1996.
  - [56] H. Oxhammar, “Document classification with uncertain data using statistical and rule-based methods,” *Uppsala University: Department of Linguistics*, 2003.
  - [57] C. Apté, F. Damerau, and S. M. Weiss, “Automated learning of decision rules for text categorization,” *ACM Transactions on Information Systems (TOIS)*, vol. 12, no. 3, pp. 233–251, 1994.
  - [58] R. Lierre, *Active learning with committees: An approach to efficient learning in text categorization using linear threshold algorithms*. Oregon State University, 2000.
  - [59] D. H. Widyantoro, T. R. Ioerger, and J. Yen, “Learning user interest dynamics with a three-descriptor representation,” *Journal of the American Society for Information Science and Technology*, vol. 52, no. 3, pp. 212–225, 2001.
  - [60] P. Rajpurkar, J. Zhang, K. Lopyrev, and P. Liang, “Squad: 100,000+ questions for machine comprehension of text,” *arXiv preprint arXiv:1606.05250*, 2016.
  - [61] G. Shen, Y. Liu, G. Tao, Q. Xu, Z. Zhang, S. An, S. Ma, and X. Zhang, “Constrained optimization with dynamic bound-scaling for effective nlp backdoor defense,” in *Int’l conf. on Machine Learning*, pp. 19879–19892, PMLR, 2022.
  - [62] R. Zellers, A. Holtzman, E. Clark, L. Qin, A. Farhadi, and Y. Choi, “Turingadvice: A generative and dynamic evaluation of language use,” *arXiv preprint arXiv:2004.03607*, 2020.
  - [63] A. Ravichander, Y. Belinkov, and E. Hovy, “Probing the probing paradigm: Does probing accuracy entail task relevance?,” *arXiv preprint arXiv:2005.00719*, 2020.
  - [64] R. Kohavi *et al.*, “Scaling up the accuracy of naive-bayes classifiers: A decision-tree hybrid,” in *Kdd*, vol. 96, pp. 202–207, 1996.
  - [65] H. Zeng, Z. Yue, Z. Kou, Y. Zhang, L. Shang, and D. Wang, “Fairness-aware training of face attribute classifiers via adversarial robustness,” *Knowledge-Based Systems*, vol. 264, p. 110356, 2023.
  - [66] X. Han, T. Baldwin, and T. Cohn, “Everybody needs good neighbours: An unsupervised locality-based method for bias mitigation,” in *The Eleventh Int’l conf. on Learning Representations*, 2023.
  - [67] M. Du, R. Tang, W. Fu, and X. Hu, “Towards debiasing dnn models from spurious feature influence,” in *Proceedings of the AAAI Conference on Artificial Intelligence*, vol. 36, pp. 9521–9528, 2022.
  - [68] R. S. Michalski, I. Mozetic, J. Hong, and N. Lavrac, “The multi-purpose incremental learning system aq15 and its testing application to three medical domains,” in *Proc. AAAI*, vol. 1986, pp. 1–041, 1986.
  - [69] K. Sullivan, A. ElMolla, B. Squires, and S. Luke, “Unlearning from demonstration,” in *Twenty-Third Int’l Joint Conference on Artificial Intelligence*, Citeseer, 2013.
  - [70] S. Gallacher, E. Papadopoulou, N. K. Taylor, and M. H. Williams, “Learning user preferences for adaptive pervasive environments: An incremental and temporal approach,” *ACM Transactions on Autonomous and Adaptive Systems (TAAS)*, vol. 8, no. 1, pp. 1–26, 2013.
  - [71] J. W. Smith, J. E. Everhart, W. Dickson, W. C. Knowler, and R. S. Johannes, “Using the adap learning algorithm to forecast the onset of diabetes mellitus,” in *Proceedings of the annual symposium on computer application in medical care*, p. 261, American Medical Informatics Association, 1988.
  - [72] A. Tuladhar, D. Rajashekar, and N. D. Forkert, “Distributed learning in healthcare,” *Trends of Artificial Intelligence and Big Data for E-Health*, pp. 183–212, 2023.
  - [73] A. Abolfazli and E. Ntoutsis, “Drift-aware multi-memory model for imbalanced data streams,” in *2020 IEEE Int’l conf. on Big Data (Big Data)*, pp. 878–885, IEEE, 2020.
  - [74] R. G. Andrzejak, K. Lehnertz, F. Mormann, C. Rieke, P. David, and C. E. Elger, “Indications of nonlinear deterministic and finite-dimensional structures in time series of brain electrical activity: Dependence on recording region and brain state,” *Physical Review E*, vol. 64, no. 6, p. 061907, 2001.
  - [75] V. S. Chundawat, A. K. Tarun, M. Mandal, and M. Kankanhalli, “Can bad teaching induce forgetting? unlearning in deep networks using an incompetent teacher,” 2022.
  - [76] D. Anguita, A. Ghio, L. Oneto, X. Parra, J. L. Reyes-Ortiz, *et al.*, “A public domain dataset for human activity recognition using smart-phones,” in *Esann*, vol. 3, p. 3, 2013.
  - [77] X. Cao, J. Jia, Z. Zhang, and N. Z. Gong, “Fedrecover: Recovering from poisoning attacks in federated learning using historical information,” *arXiv preprint arXiv:2210.10936*, 2022.
  - [78] L. Song, *Understanding and Measuring Privacy Risks in Machine Learning*. PhD thesis, Princeton University, 2021.
  - [79] W. Hu, M. Fey, M. Zitnik, Y. Dong, H. Ren, B. Liu, M. Catasta, and J. Leskovec, “Open graph benchmark: Datasets for machine learning on graphs,” *Advances in neural information processing systems*, vol. 33, pp. 22118–22133, 2020.
  - [80] P. Tarau, “A gaze into the internal logic of graph neural networks, with logic,” *arXiv preprint arXiv:2208.03093*, 2022.
  - [81] P. Sen, G. Namata, M. Bilgic, L. Getoor, B. Gallagher, and T. Eliassi-Rad, “Collective classification in network data,” *AI magazine*, vol. 29, no. 3, pp. 93–93, 2008.
  - [82] H. Hu, Z. Salicic, L. Sun, G. Dobbie, P. S. Yu, and X. Zhang, “Membership inference attacks on machine learning: A survey,” *ACM Computing Surveys (CSUR)*, vol. 54, no. 11s, pp. 1–37, 2022.
  - [83] E. Chien, C. Pan, and O. Milenkovic, “Efficient model updates for approximate unlearning of graph-structured data,” in *The Eleventh Int’l conf. on Learning Representations*, 2023.
  - [84] X. Zhang, J. Zhao, and Y. LeCun, “Character-level convolutional networks for text classification,” *Advances in neural information processing systems*, vol. 28, 2015.
  - [85] D. M. Sommer, L. Song, S. Wagh, and P. Mittal, “Athena: Probabilistic verification of machine unlearning,” *Proceedings on Privacy Enhancing Technologies*, vol. 3, pp. 268–290, 2022.
  - [86] M. A. A. Gonzalez, M. J. Abe, B. F. Amadeu, S. L. Sayuri, *et al.*, “Pann component for use in pattern recognition in medical diagnostics decision-making,” *Procedia Computer Science*, vol. 192, pp. 1750–1759, 2021.
  - [87] H. Xiao, K. Rasul, and R. Vollgraf, “Fashion-mnist: a novel image dataset for benchmarking machine learning algorithms,” *arXiv preprint arXiv:1708.07747*, 2017.
  - [88] K. Chen, Y. Huang, and Y. Wang, “Machine unlearning via gan,” *arXiv preprint arXiv:2111.11869*, 2021.
  - [89] Y. Liu, G. Shen, G. Tao, Z. Wang, S. Ma, and X. Zhang, “Complex backdoor detection by symmetric feature differencing,” in *Proceedings of the IEEE/CVF Conference on Computer Vision and Pattern Recognition*, pp. 15003–15013, 2022.
  - [90] J. H. Lee, “Dynmat, a network that can learn after learning,” *Neural Networks*, vol. 116, pp. 88–100, 2019.
  - [91] S. Lee, W. Song, S. Jana, M. Cha, and S. Son, “Evaluating the robustness of trigger set-based watermarks embedded in deep neural networks,” *IEEE Transactions on Dependable and Secure Computing*, 2022.
  - [92] L. Fei-Fei, R. Fergus, and P. Perona, “Learning generative visual models from few training examples: An incremental bayesian approach tested on 101 object categories,” in *2004 conference on computer vision and pattern recognition workshop*, pp. 178–178, IEEE, 2004.
  - [93] M. Du, Z. Chen, C. Liu, R. Oak, and D. Song, “Lifelong anomaly detection through unlearning,” in *Proceedings of the 2019 ACM SIGSAC Conference on Computer and Communications Security*, pp. 1283–1297, 2019.
  - [94] S. S. Shivagunde and V. V. Saradhi, “View incremental decremental multi-view discriminant analysis,” *Applied Intelligence*, pp. 1–15, 2022.
  - [95] T. Diethe and M. Girolami, “Online learning with (multiple) kernels: A review,” *Neural computation*, vol. 25, no. 3, pp. 567–625, 2013.
  - [96] T.-Y. Lin, M. Maire, S. Belongie, J. Hays, P. Perona, D. Ramanan, P. Dollár, and C. L. Zitnick, “Microsoft coco: Common objects in context,” in *Computer Vision—ECCV 2014: 13th European Conference, Zurich, Switzerland, September 6–12, 2014, Proceedings, Part V 13*, pp. 740–755, Springer, 2014.
  - [97] E. Zhang, K. Wang, X. Xu, Z. Wang, and H. Shi, “Forget-me-not: Learning to forget in text-to-image diffusion models,” *arXiv preprint arXiv:2303.17591*, 2023.

- [98] S. Yu, J. Guo, R. Zhang, Y. Fan, Z. Wang, and X. Cheng, "A re-balancing strategy for class-imbalanced classification based on instance difficulty," in *Proceedings of the IEEE/CVF Conference on Computer Vision and Pattern Recognition*, pp. 70–79, 2022.
- [99] A. Hoblitzell, M. Babbar-Sebens, and S. Mukhopadhyay, "Uncertainty-based deep learning networks for limited data wetland user models," in *2018 IEEE Int'l conf. on Artificial Intelligence and Virtual Reality (AIVR)*, pp. 19–26, IEEE, 2018.
- [100] J. Autz, S. K. Mishra, L. Herrmann, and J. Hertzberg, "The pitfalls of transfer learning in computer vision for agriculture," *42. GIL-Jahrestagung, Künstliche Intelligenz in der Agrar-und Ernährungswirtschaft*, 2022.
- [101] H. Bansal, N. Singhi, Y. Yang, F. Yin, A. Grover, and K.-W. Chang, "Cleanclip: Mitigating data poisoning attacks in multimodal contrastive learning," in *ICLR 2023 Workshop on Trustworthy and Reliable Large-Scale Machine Learning Models*.
- [102] L. Wolf, T. Hassner, and I. Maoz, "Face recognition in unconstrained videos with matched background similarity," in *CVPR 2011*, pp. 529–534, IEEE, 2011.
- [103] A. Bendale and T. Boulton, "Reliable posterior probability estimation for streaming face recognition," in *Proceedings of the IEEE Conference on Computer Vision and Pattern Recognition Workshops*, pp. 56–63, 2014.
- [104] S. Kaviani and I. Sohn, "Defense against neural trojan attacks: A survey," *Neurocomputing*, vol. 423, pp. 651–667, 2021.
- [105] Y. Zhao, H. Zhu, K. Chen, and S. Zhang, "Ai-lancet: Locating error-inducing neurons to optimize neural networks," in *Proceedings of the 2021 ACM SIGSAC Conference on Computer and Communications Security*, pp. 141–158, 2021.
- [106] A. K. Veldanda, K. Liu, B. Tan, P. Krishnamurthy, F. Khorrami, R. Karri, B. Dolan-Gavitt, and S. Garg, "Nnoculation: Catching badnets in the wild," in *Proceedings of the 14th ACM Workshop on Artificial Intelligence and Security*, pp. 49–60, 2021.
- [107] I. Serna, A. Morales, J. Fierrez, and N. Obradovich, "Sensitive loss: Improving accuracy and fairness of face representations with discrimination-aware deep learning," *Artificial Intelligence*, vol. 305, p. 103682, 2022.
- [108] P. Helber, B. Bischke, A. Dengel, and D. Borth, "Eurosat: A novel dataset and deep learning benchmark for land use and land cover classification," *IEEE Journal of Selected Topics in Applied Earth Observations and Remote Sensing*, vol. 12, no. 7, pp. 2217–2226, 2019.
- [109] L. Risser, A. Picard, L. Hervier, and J.-M. Loubes, "A survey of identification and mitigation of machine learning algorithmic biases in image analysis," *arXiv preprint arXiv:2210.04491*, 2022.
- [110] C. O. Sakar, S. O. Polat, M. Katircioglu, and Y. Kastro, "Real-time prediction of online shoppers' purchasing intention using multilayer perceptron and lstm recurrent neural networks," *Neural Computing and Applications*, vol. 31, pp. 6893–6908, 2019.
- [111] S. Mercuri, R. Khraishi, R. Okhrati, D. Batra, C. Hamill, T. Ghasem-pour, and A. Nowlan, "An introduction to machine unlearning," *arXiv preprint arXiv:2209.00939*, 2022.
- [112] J. Weng, S. Yao, Y. Du, J. Huang, J. Weng, and C. Wang, "Proof of unlearning: Definitions and instantiation," *arXiv preprint arXiv:2210.11334*, 2022.
- [113] K. Koch and M. Soll, "No matter how you slice it: Machine unlearning with sisa comes at the expense of minority classes," in *First IEEE Conference on Secure and Trustworthy Machine Learning*.
- [114] Y. He, G. Meng, K. Chen, J. He, and X. Hu, "Deepoblivate: a powerful charm for erasing data residual memory in deep neural networks," *arXiv preprint arXiv:2105.06209*, 2021.
- [115] N. Su and B. Li, "Asynchronous federated unlearning,"
- [116] D. Anguita, A. Ghio, L. Oneto, X. Parra, and J. L. Reyes-Ortiz, "Human activity recognition on smartphones using a multiclass hardware-friendly support vector machine," in *Ambient Assisted Living and Home Care: 4th Int'l Workshop, IWAAL 2012, Vitoria-Gasteiz, Spain, December 3-5, 2012. Proceedings 4*, pp. 216–223, Springer, 2012.
- [117] M. N. K. Boulos and S. P. Yang, "Mobile physical activity planning and tracking: a brief overview of current options and desiderata for future solutions," *Mhealth*, vol. 7, 2021.
- [118] F. M. Harper and J. A. Konstan, "The movielens datasets: History and context," *ACM Trans. Interact. Intell. Syst.*, vol. 5, Dec. 2015.
- [119] Z. Chen, F. Sun, Y. Tang, H. Chen, J. Gao, and B. Ding, "Studying the impact of data disclosure mechanism in recommender systems via simulation," *ACM Transactions on Information Systems*, vol. 41, no. 3, pp. 1–26, 2023.
- [120] Z. Chen, F. Sun, Y. Tang, H. Chen, J. Gao, and B. Ding, "Proactively control privacy in recommender systems," *arXiv preprint arXiv:2204.00279*, 2022.
- [121] C. Ganhör, D. Penz, N. Rekabsaz, O. Lesota, and M. Schedl, "Unlearning protected user attributes in recommendations with adversarial training," in *Proceedings of the 45th Int'l ACM SIGIR Conference on Research and Development in Information Retrieval*, pp. 2142–2147, 2022.
- [122] Y. Yao, C. Wang, and H. Li, "Learning to counterfactually explain recommendations," *arXiv preprint arXiv:2211.09752*, 2022.
- [123] W. Yuan, H. Yin, F. Wu, S. Zhang, T. He, and H. Wang, "Federated unlearning for on-device recommendation," in *Proceedings of the 16th ACM Int'l conf. on Web Search and Data Mining*, pp. 393–401, 2023.
- [124] M. Xu, J. Sun, X. Yang, K. Yao, and C. Wang, "Netflix and forget: Efficient and exact machine unlearning from bi-linear recommendations," *arXiv preprint arXiv:2302.06676*, 2023.
- [125] B. Omidvar-Tehrani and S. Amer-Yahia, "User group analytics survey and research opportunities," *IEEE Transactions on Knowledge and Data Engineering*, vol. 32, no. 10, pp. 2040–2059, 2019.
